# Supplementary material for: Compositional Servoing by Recombining Demonstrations
Source: arXiv:2310.04271 source file (2023-10-06)
Supplement: Supplementary file 1 [file 7_supplement.tex]

%%%%%%%%%% Merge with supplemental materials %%%%%%%%%%
\clearpage

\setlength{\belowcaptionskip}{0pt}

\begin{strip}
\begin{center}
\vspace{-5ex}
\textbf{\LARGE \bf
Compositional Servoing by Recombining Demonstrations} \\
\vspace{3ex}

\Large{\bf- Supplementary Material -}\\
 \vspace{0.4cm}
 \normalsize{Abhijeet Nayak,
HiWi?,
Martin Büchner,
Silvio Galesso,
Max Argus,
Abhinav Valada,
and Thomas Brox}
\end{center}
\end{strip}

%%%%%%%%%% Merge with supplemental materials %%%%%%%%%%
\setcounter{section}{0}
\setcounter{equation}{0}
\setcounter{figure}{0}
\setcounter{table}{0}
\setcounter{page}{1}
\makeatletter

%%%%%%%%%% Prefix a "S" to all equations, figures, tables and reset the counter %%%%%%%%%%

 \footnote{$^{*}$ Equal contribution.\\
 $^{1}$ Department of Computer Science, University of Freiburg, Germany.\\
% Project page: \url{http://curb.cs.uni-freiburg.de}
 }%
\normalsize

\section{Similarity Function evaluation}

\begin{table}[htb]
    \scriptsize
    \centering
    \label{tab:init_estimate}
    \begin{threeparttable}
        \begin{tabular}{l|c|c|c}
        \toprule
            Experiment & Function & Position & Orientation \\
             & & MSE (cm) & MSE (rad) \\
            \midrule
            Long-Horizon & FlowControl & 7.7 & 0.242 \\
             & HLOC & \textbf{5.8} & \textbf{0.184} \\
            \midrule
            Next Action & VS & \textbf{3.6} & 0.015 \\ 
             & VINN & 4.8 & 0.014 \\
             & R3M & 5.7 & \textbf{0.013} \\
            
            \bottomrule
        \end{tabular}
        \footnotesize
        Position and Orientation errors on long-horizon and next actions.
        For the long-horizon task, we compare the Visual Similarity function (VS) and Hierarchical Localization (HLOC) while using the initial transformation estimates from the respective functions. 
        while comparing the next action, we use VINN and the Visual Similarity function.
        HLOC performs better in the first task, whereas the visual similarity function demonstrates lower error in the latter. We compute these scores over 30 episodes of offline data.\todo{Include R3M in this table?}
    \end{threeparttable}
\end{table}
